# Supplementary material for: Mobile authentication of copy detection patterns
Source: arXiv:2203.02397 source file (2022-05-18)
Supplement: Supplementary file 1 [file decomposition_tricks.tex]

% ----------------------------------------
\section{Mutual information decomposition tricks}
\label{app:mutual info decomposition tricks}

According to the definition (\ref{ib-sup second term direct decomposition}) in Section \ref{subsubsec: sup class second term}, the mutual information  $I(\A; \C)$ can be decomposed as:
\begin{equation}
\begin{aligned} 
	I(\A; \C) & = \mathbb{E}_{\pac}  \left[  \log \frac{p(\c| \a)}{p(\c)}  \right] \\
              & = - \mathbb{E}_{p(\c)}  \left[  \log p(\c)\right] + \mathbb{E}_{\pac}  \left[  \log p(\c| \a)\right].
 \end{aligned} 
\label{ib-occ second term direct decomposition app}
\end{equation}
The first term of this decomposition corresponds to the entropy of class labels $H(\C) =\;$ $- \mathbb{E}_{p(\c)}  \left[ \log p(\c) \right]$. In the second term the transition probability $p(\c| \a)$ is unknown. At the same time, it can be written as:
\begin{equation}
\begin{aligned} 
\mathbb{E}_{\pac} \left[ \log p(\c|\a)\right] & =   \int_{\c}\int_{\a}  p(\a, \c)   \log p(\c|\a)   \ d\c \ d\a.
\end{aligned} 
\label{MI_2nd_unsupervised_cond_entropy1} 
\end{equation}
The expectation with respect to the joint distribution $\pac$ can also be defined via the marginalization $\pac = \int_{\x} p(\x,\a,\c)d\x = \int_{\x} p(\c, \x)q_{\bphi}(\a|\x) d\x$. Combing these results, one can obtain:    
%
%
%\begin{equation}
\begin{multline}
    \mathbb{E}_{p(\a,\c)}  \left[  \log p(\c| \a)\right] =  \\
    = \int_{\c}\int_{\a}\int_{\x}  p(\c,\x) q_{\bphi}(\a|\x)  \log p(\c|\a) \ d\c  \ d\a \ d\x \\ 
    = \mathbb{E}_{p(\c, \x)}  \left[   \mathbb{E}_{q_{\bphi}(\a|\x)} \left[  \log p(\c| \a) \right]\right].
\label{MI_2nd_unsupervised_cond_entropy2}    
\end{multline}
%\label{MI_2nd_unsupervised_cond_entropy2}
%\end{equation}
%
%
To overcome the problem of unknown $p(\c| \a)$, a variational distribution $p_{\btheta}(\c| \a)$ parametrized via a set of parameters $\btheta$ is applied to approximate $p(\c| \a)$:
\begin{equation}
 \begin{aligned} 
\label{MI_2nd_unsupervised_cond_entropy3}
    \mathbb{E}_{p(\a,\c)}  \left[  \log p(\c| \a)\right]  
    & =   \mathbb{E}_{p(\c,{\bf x} )}  \left[   \mathbb{E}_{q_{\bphi}(\a|{\bf x})} \left[  \log p(\c| \a) \frac{ p_{\btheta}(\c| \a)}{p_{\btheta}(\c| \a)} \right]\right] \\ 
    & = \mathbb{E}_{p(\c,{\bf x} )}  \left[   \mathbb{E}_{q_{\bphi}(\a|{\bf x})} \left[  \log p_{\btheta}(\c| \a) \right]\right] \\
    & \;\;\; + \mathbb{E}_{p(\a,\c)}  \left[ \log  \frac{p(\c| \a)}{p_{\btheta}(\c| \a)} \right],
 \end{aligned}
\end{equation}
where in the second term the expectation defined in (\ref{MI_2nd_unsupervised_cond_entropy2}) is used. 
%
%\begin{equation}
\begin{multline} 
    \mathbb{E}_{p(\a,\c )}  \left[ \log  \frac{p(\c| \a)}{p_{\btheta}(\c| \a)} \right] = \mathbb{E}_{p(\a )} \left[  \mathbb{E}_{p(\c|\a )}   \left[ \log  \frac{p(\c| \a)}{p_{\btheta}(\c| \a)} \right]\right] \\ 
    =  \mathbb{E}_{p(\a)} \left[D_{\mathrm{KL}}\left(p(\c|\A=\a) \| p_{\btheta}(\c|\A=\a)\right)  \right] \\ 
    = D_{\mathrm{KL}}\left(p(\c|\a ) \| p_{\btheta}(\c|\a)\right).
\label{MI_2nd_unsupervised_cond_entropy4}
\end{multline} 
%\end{equation}
%
%
Since the KL-divergence $D_{\mathrm{KL}}\left(p(\c|\a ) \| p_{\btheta}(\c|\a)\right) \geq 0$, the (\ref{MI_2nd_unsupervised_cond_entropy3}) can be lower bounded as:
\begin{equation}
\begin{aligned}
\mathbb{E}_{p(\a,\c)}  \left[  \log p(\c| \a)\right]  & \geq \mathbb{E}_{p(\c,\x )}  \left[ \mathbb{E}_{q_{\bphi}(\a|\x)} \left[  \log p_{\btheta}(\c| \a) \right]\right].
\end{aligned}
\label{MI_2nd_unsupervised_cond_entropy5}
\end{equation}
Therefore, the mutual information (\ref{ib-occ second term direct decomposition app}) can be lower bounded as  $I(\A; \C) \geq I_{\btheta, \bphi_\rma}(\A;\C)$, where the lower bound is defined as:
\begin{equation}
\begin{aligned} 
    I_{\btheta, \bphi_\rma}(\A;\C) & \triangleq H(\C) + \mathbb{E}_{p(\c,\x )}  \left[   \mathbb{E}_{q_{\bphi}(\a|\x)} \left[  \log p_{\btheta}(\c| \a) \right]\right]
 \\ & = H(\C) - H_{\btheta, \bphi_\rma} (\C|\A),
\end{aligned} 
\label{IB_S_lower_bound1}
\end{equation}
where $H_{\btheta, \bphi_\rma} (\C|\A) = - \mathbb{E}_{p(\c,\x )}  \left[\mathbb{E}_{q_{\bphi}(\a|\x)} \left[  \log p_{\btheta}(\c| \a) \right]\right]$.
