# Supplementary material for: Mobile authentication of copy detection patterns
Source: arXiv:2203.02397 source file (2022-05-18)
Supplement: Supplementary file 2 [file spatial_domain.tex]

\section{Spatial domain analysis}
\label{app:spatial domain analysis}

%--- One metric digital vs physical ---------------------------
\begin{figure}[h!]
	\centering
	\begin{subfigure}{0.48\columnwidth}
		\centering
		\captionsetup{justification=centering}
        \includegraphics[width=1\linewidth,valign=t]{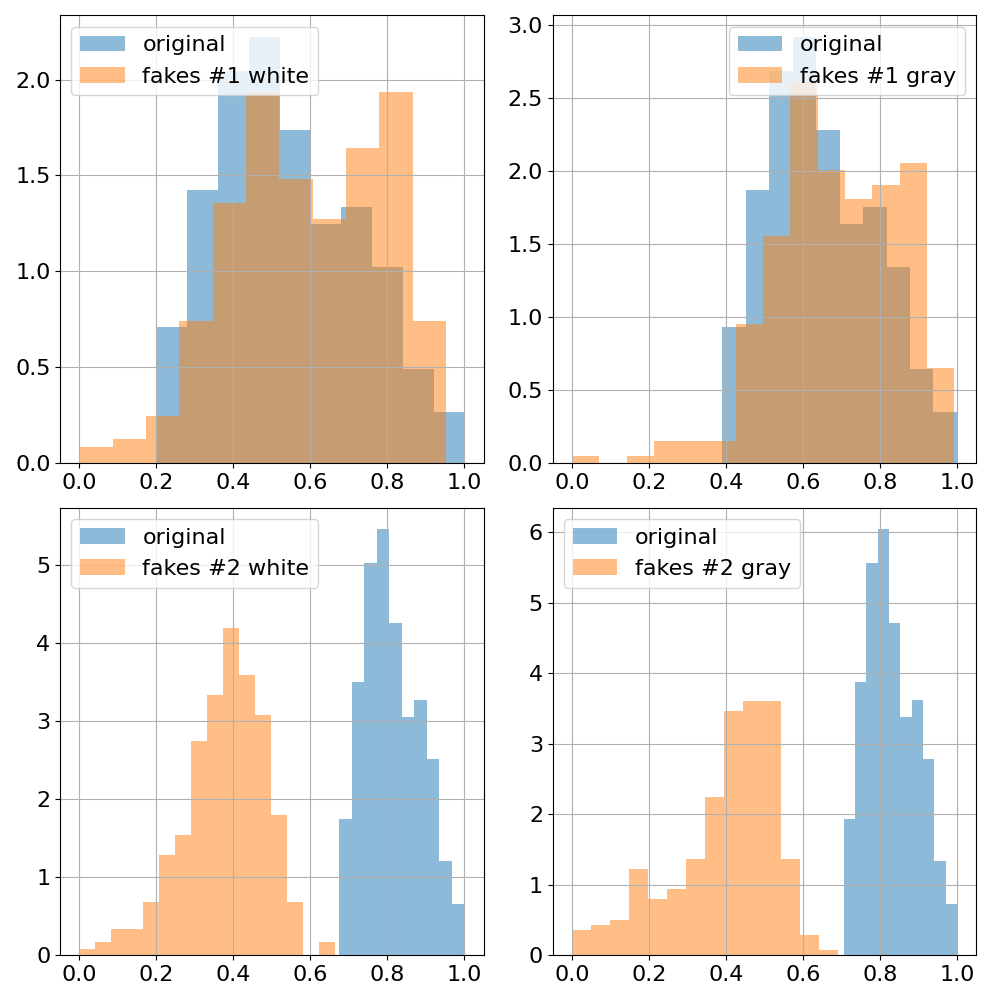}
	    \caption{Pearson correlation with respect to \\ the digital templates/references.}
	    \label{fig:spatial domain digital pearson gray main}
	\end{subfigure}		
	%
	%%\hspace{0.2cm}
	%
	\begin{subfigure}{0.48\columnwidth}
		\centering
		\captionsetup{justification=centering}		
        \includegraphics[width=1\linewidth,valign=t]{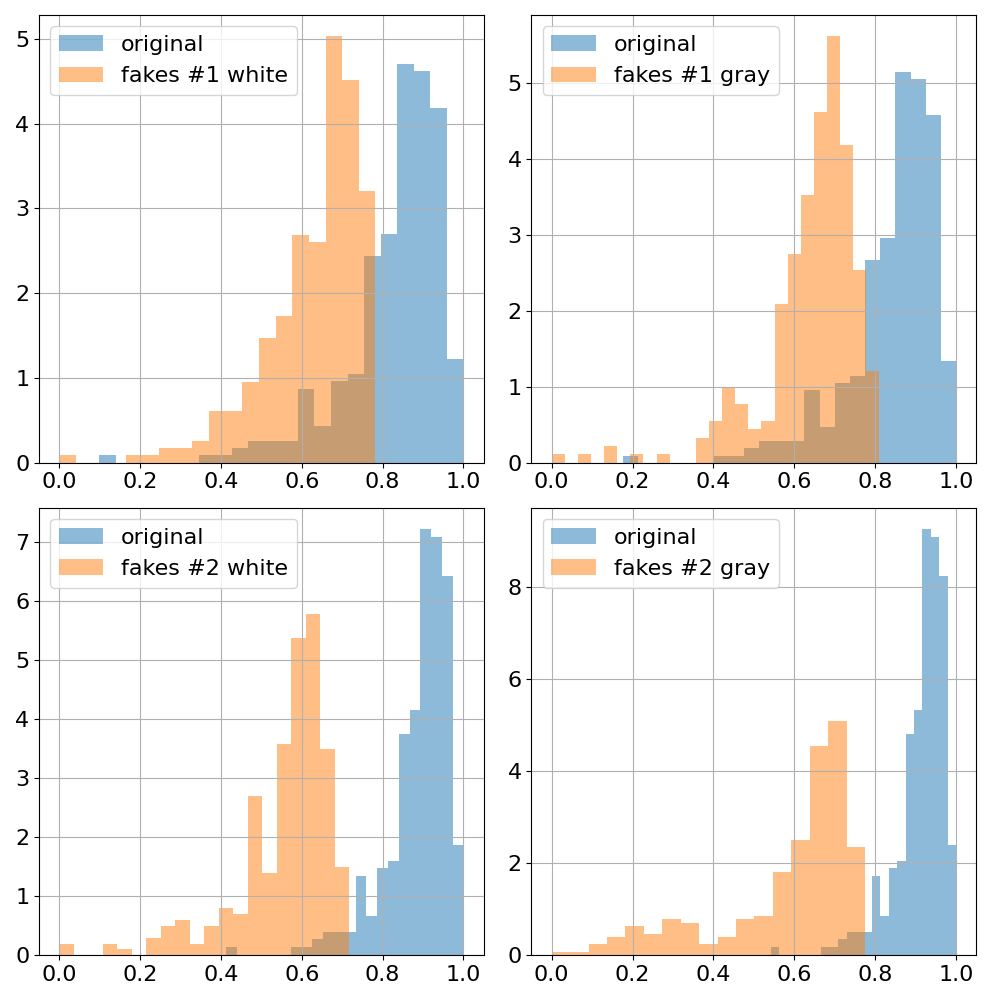}
	    \caption{Pearson correlation with respect to \\the physical references.}
	    \label{fig:spatial domain physical pearson rgb main}
	\end{subfigure}		
	\\ [1cm]
	\begin{subfigure}{0.48\columnwidth}
		\centering
		\captionsetup{justification=centering}
        \includegraphics[width=1\linewidth,valign=t]{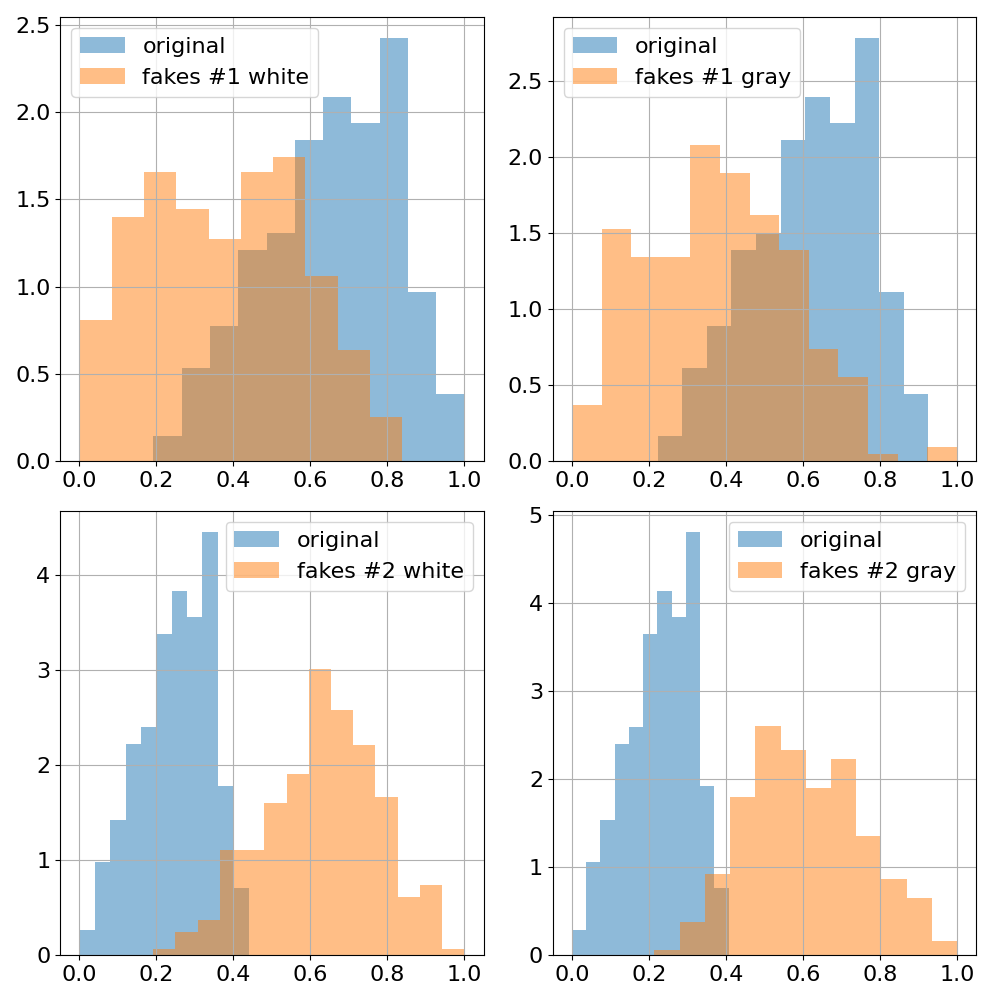}
	    \caption{Hamming distance with respect to \\ the digital templates/references.}
	    \label{fig:spatial domain digital xor otsu gray main}
	\end{subfigure}		
	%
	%%\hspace{0.2cm}
	%
	\begin{subfigure}{0.48\columnwidth}
		\centering
		\captionsetup{justification=centering}
        \includegraphics[width=1\linewidth,valign=t]{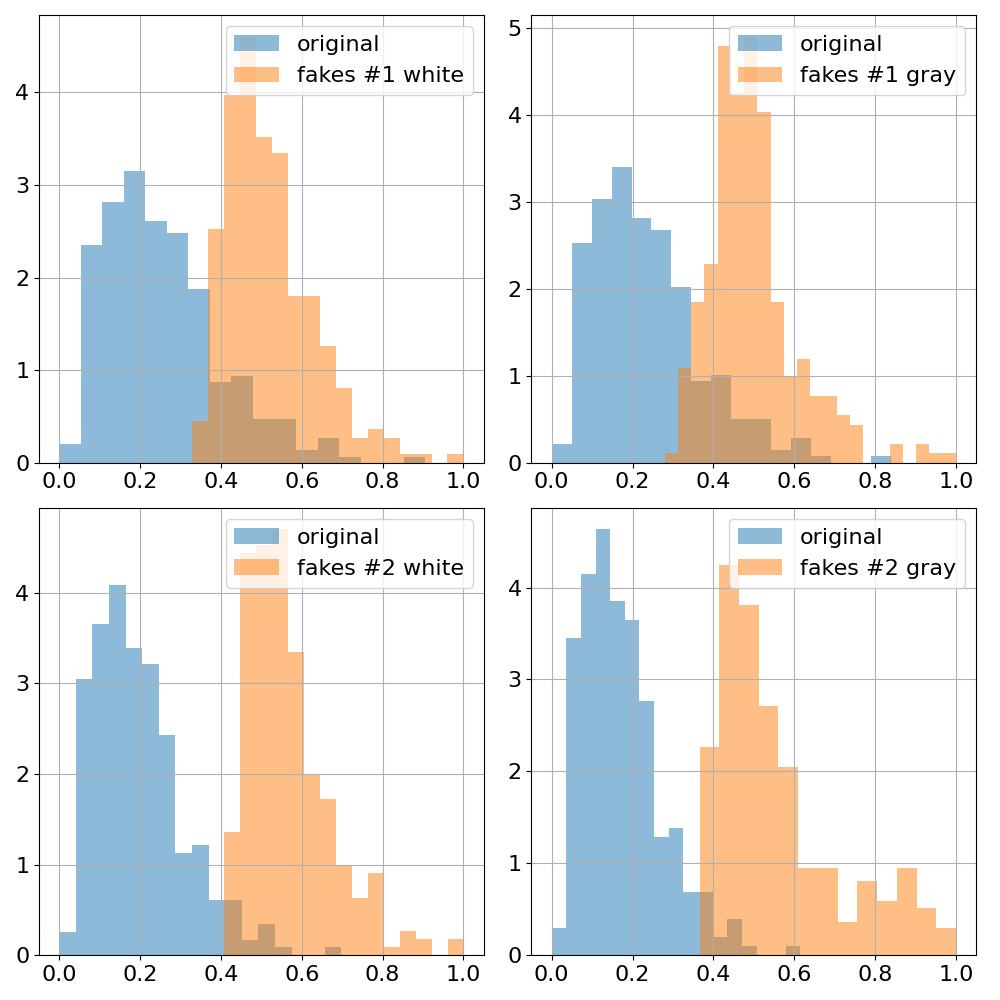}
	    \caption{Hamming distance with respect to \\ the binarized physical references.}
	    \label{fig:spatial domain physical xor otsu rgb main}
	\end{subfigure}		
	\\ [1cm]
    \caption{The distribution of the Hamming  distances between the references (digital or physical) and the corresponding printed codes (original and fakes). In case of the physical references the binarization is applied as a simple thresholding with an optimal threshold determined individually for each code via Otsu's method.}
    \label{fig:spatial domain digital vs physical one metric main}        
\end{figure}

%------------------------------

%--- One meteric 1 ---------------------------
\begin{figure}[h!]
	\centering
	
	\begin{subfigure}{0.48\columnwidth}
		\centering
		\captionsetup{justification=centering}
        \includegraphics[width=1\linewidth,valign=t]{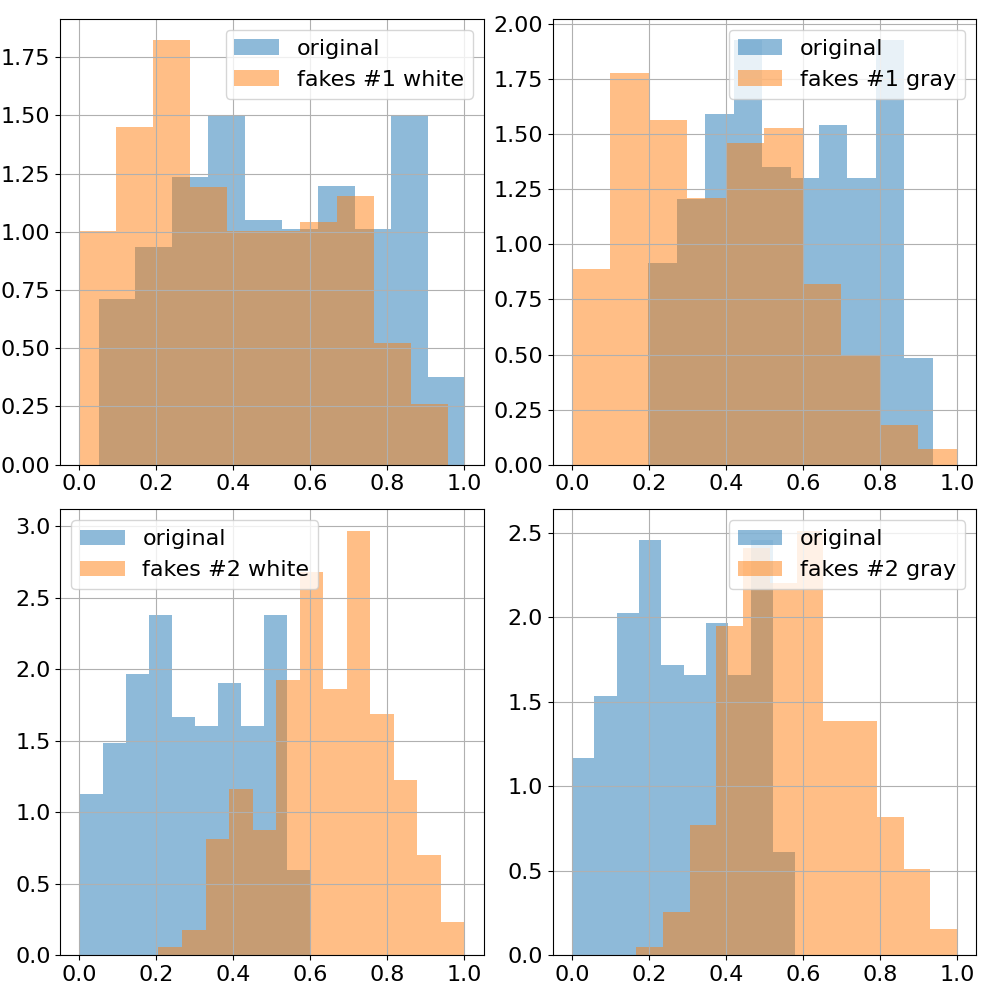}
	    \caption{$\ell_1$ distance with respect to \\ the digital templates/references.}
	    \label{fig:spatial domain digital l1 rgb}
	\end{subfigure}		
	%
	%\hspace{0.2cm}
	%
	\begin{subfigure}{0.48\columnwidth}
		\centering
		\captionsetup{justification=centering}
        \includegraphics[width=1\linewidth,valign=t]{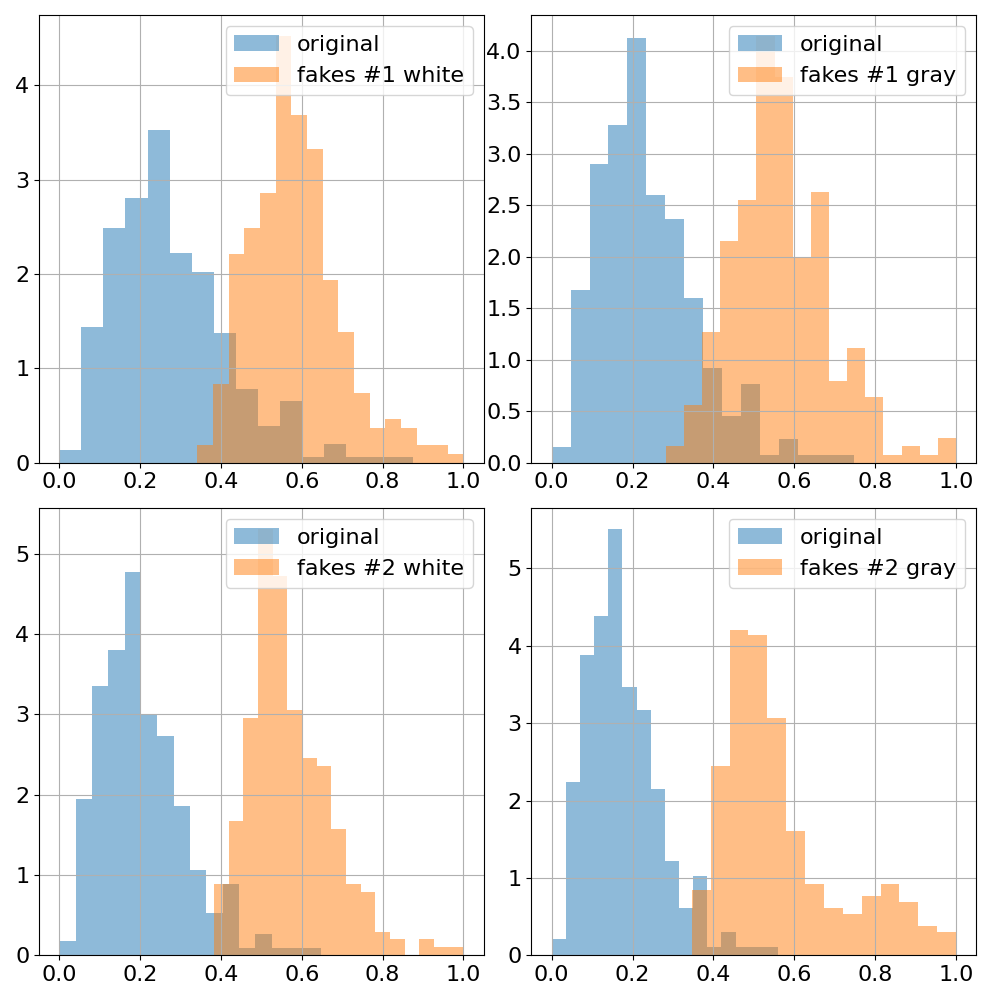}
	    \caption{$\ell_1$ distance with respect to \\ the physical reference.}
	    \label{fig:spatial domain physical l1 rgb}
	\end{subfigure}	
	\\ [0.6cm]
	\begin{subfigure}{0.48\columnwidth}
		\centering
		\captionsetup{justification=centering}		
        \includegraphics[width=1\linewidth,valign=t]{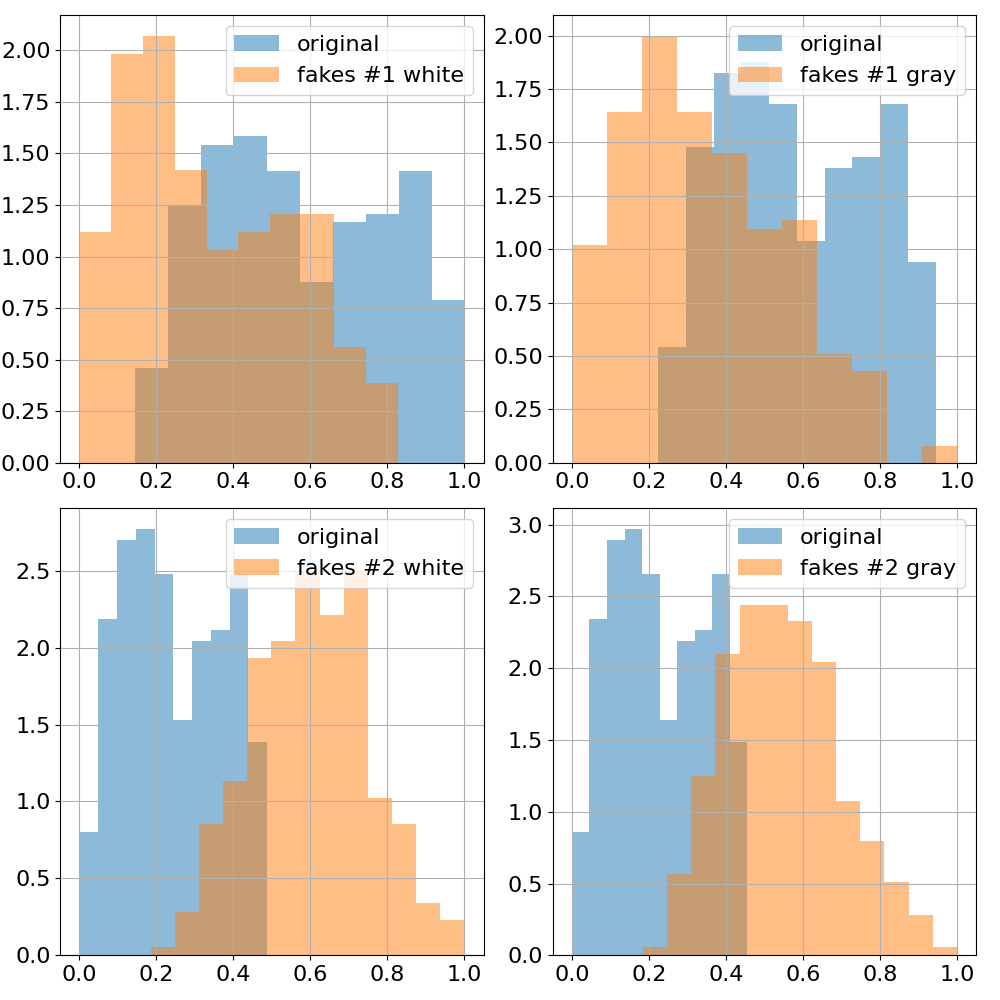}
	    \caption{$\ell_2$ distance with respect to \\ the digital templates/references.}
	    \label{fig:spatial domain digital l2 rgb}
	\end{subfigure}		
	%
	%\hspace{0.2cm}
	%
	\begin{subfigure}{0.48\columnwidth}
		\centering
		\captionsetup{justification=centering}		
        \includegraphics[width=1\linewidth,valign=t]{appendices/spatial_domain/one_metrics/rgb_phisical_references_l1_330_x_330_normalised.png}
	    \caption{$\ell_2$ distance with respect to \\ the physical reference.}
	    \label{fig:spatial domain physical l2 rgb}
	\end{subfigure}		
	\\ [0.6cm]
    \caption{The distribution of the $\ell_1$ and $\ell_2$ distances between the references (digital or physical) and the corresponding printed codes (original and fakes).}
    \label{fig:spatial domain digital l1 l2 metric digital vs physical}        
\end{figure}

%------------------------------

%--- Two metric 1 ---------------------------
\begin{figure}[h!]
	\centering
	\begin{subfigure}{0.49\columnwidth}
		\centering
		\captionsetup{justification=centering}		
        \includegraphics[width=0.975\linewidth,valign=t]{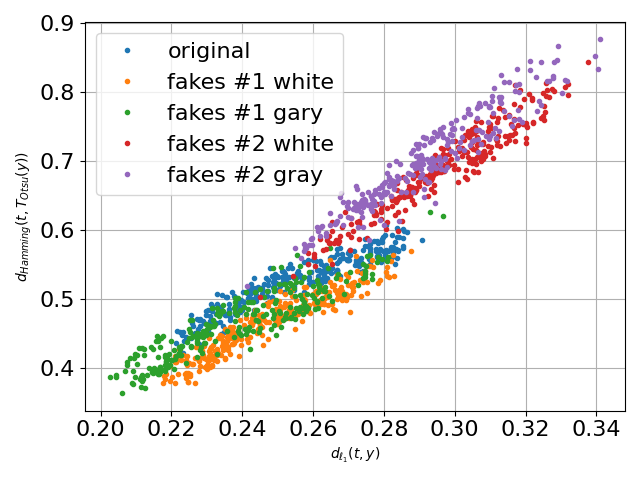}
	    \caption{$\ell_1$ vs Hamming distance with respect \\ to the digital templates/references.}
	    \label{fig:spatial domain gray l1 vs xor otsu digital}
	\end{subfigure}		
	\begin{subfigure}{0.49\columnwidth}
		\centering
		\captionsetup{justification=centering}		
        \includegraphics[width=0.975\linewidth,valign=t]{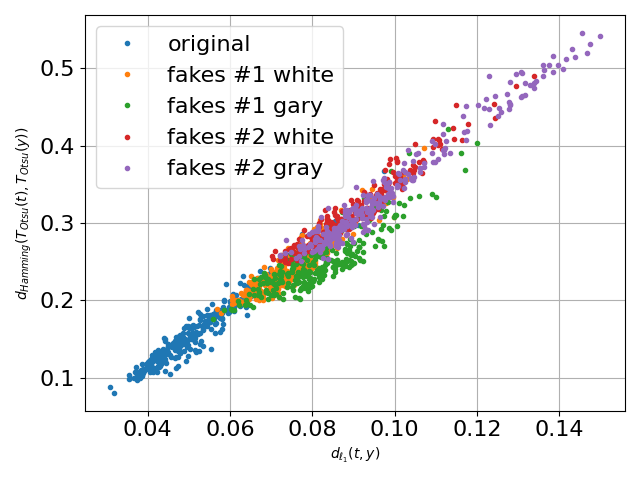}
	    \caption{$\ell_1$ vs Hamming distance with respect \\ to the physical references.}
	    \label{fig:spatial domain rgb l1 vs xor otsu physical}
	\end{subfigure}		
	\\ % --- raw 2 ----
	\begin{subfigure}{0.49\columnwidth}
		\centering
		\captionsetup{justification=centering}		
        \includegraphics[width=0.975\linewidth,valign=t]{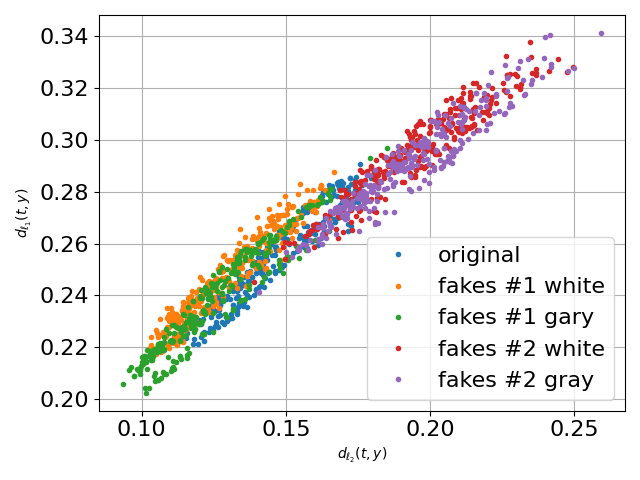}
	    \caption{$\ell_2$ vs $\ell_1$ distances with respect \\ to the digital templates/references.}
	    \label{fig:spatial domain gray l1 vs l2 digital}
	\end{subfigure}		
	\begin{subfigure}{0.49\columnwidth}
		\centering
		\captionsetup{justification=centering}		
        \includegraphics[width=0.975\linewidth,valign=t]{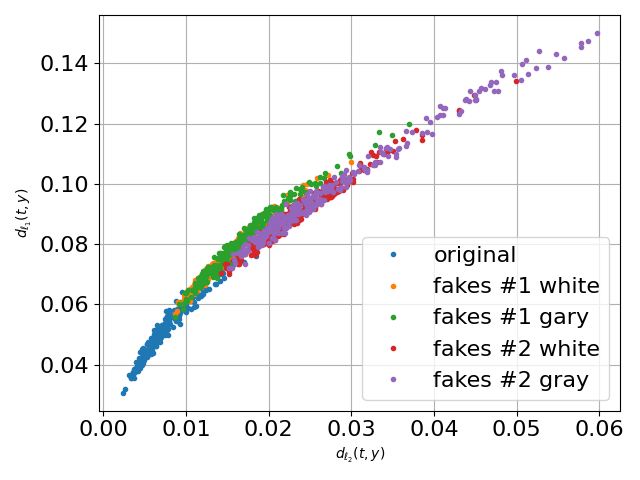}
	    \caption{$\ell_2$ vs $\ell_1$ distances with respect \\ to the physical references.}
	    \label{fig:spatial domain rgb l1 vs l2 physical}
	\end{subfigure}		
	\\ % --- raw 3 ----
	\begin{subfigure}{0.49\columnwidth}
		\centering
		\captionsetup{justification=centering}		
        \includegraphics[width=0.975\linewidth,valign=t]{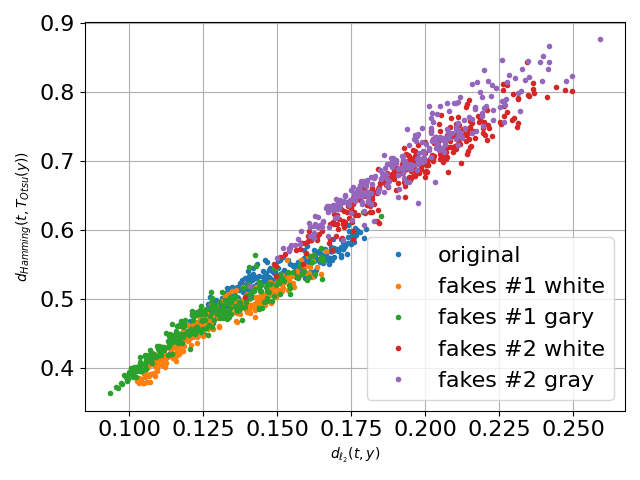}
	    \caption{$\ell_2$ vs Hamming distance with respect \\ to the digital templates/references.}
	    \label{fig:spatial domain gray l2 vs xor otsu digital}
	\end{subfigure}		
	\begin{subfigure}{0.49\columnwidth}
		\centering
		\captionsetup{justification=centering}		
        \includegraphics[width=0.975\linewidth,valign=t]{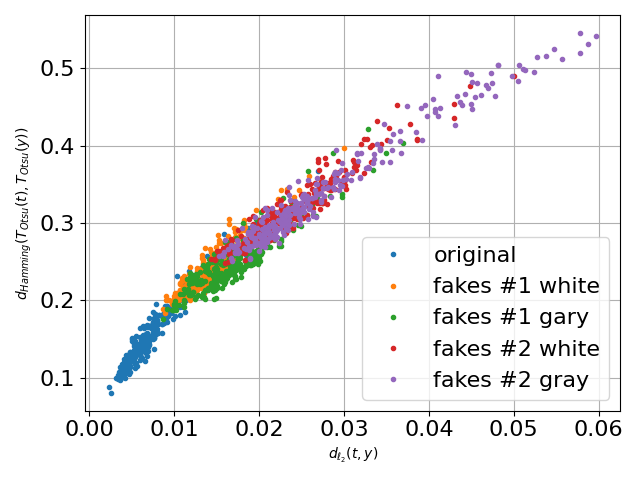}
	    \caption{$\ell_2$ vs Hamming distance with respect \\ to the physical references.}
	    \label{fig:spatial domain rgb l2 vs xor otsu physical}
	\end{subfigure}		
	\\
    \caption{The 2D PGC separability in the spatial domain with respect to the $\ell_2$, $\ell_1$ and Hamming distances between the references (digital or physical) and the corresponding printed codes (original and fakes) (part 1).}
    \label{fig:spatial domain two metric part 1}        
\end{figure}

%------------------------------
%--- Two metric 2 ---------------------------
\begin{figure}[h!]
	\centering
	\begin{subfigure}{0.49\columnwidth}
		\centering
		\captionsetup{justification=centering}		
        \includegraphics[width=0.975\linewidth,valign=t]{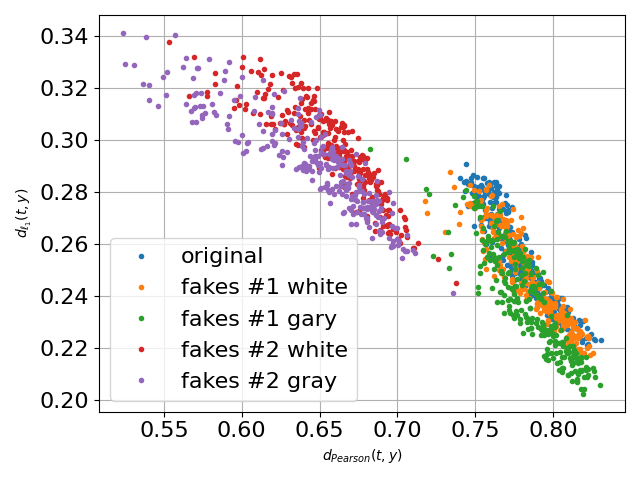}
	    \caption{Pearson correlation vs $\ell_1$ distance with \\ respect to the digital templates/references.}
	    \label{fig:spatial domain gray pearson vs l1 digital}
	\end{subfigure}		
	\begin{subfigure}{0.49\columnwidth}
		\centering
		\captionsetup{justification=centering}		
        \includegraphics[width=0.975\linewidth,valign=t]{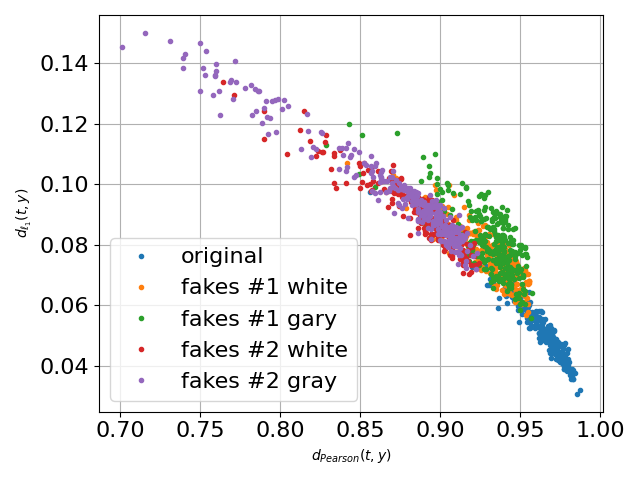}
	    \caption{Pearson correlation vs $\ell_1$ distance with \\ respect to the physical references.}
	    \label{fig:spatial domain rgb pearson vs l1 physical}
	\end{subfigure}		
	\\ % --- raw 2 ----
	\begin{subfigure}{0.49\columnwidth}
		\centering
		\captionsetup{justification=centering}		
        \includegraphics[width=0.975\linewidth,valign=t]{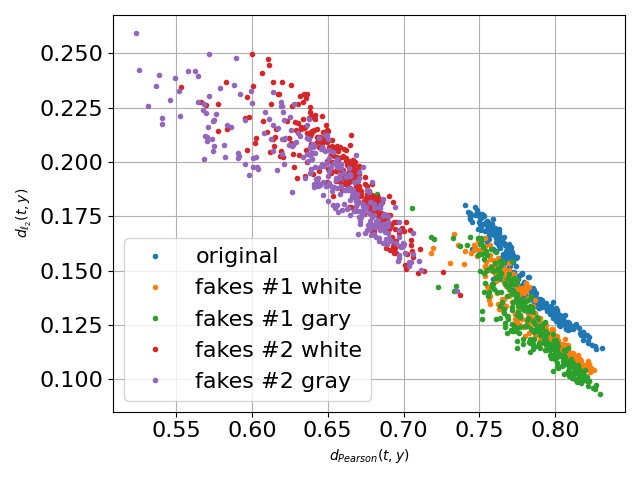}
	    \caption{Pearson correlation vs $\ell_2$ distance with \\ respect to the digital templates/references.}
	    \label{fig:spatial domain gray pearson vs l2 digital}
	\end{subfigure}		
	\begin{subfigure}{0.49\columnwidth}
		\centering
		\captionsetup{justification=centering}		
        \includegraphics[width=0.975\linewidth,valign=t]{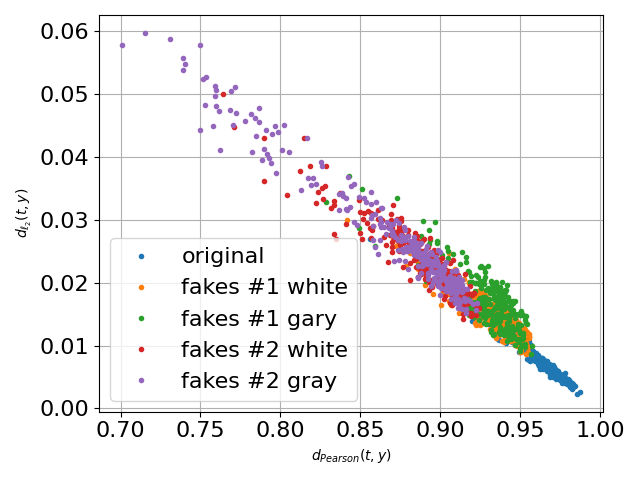}
	    \caption{Pearson correlation vs $\ell_2$ distance with \\ respect to the physical references.}
	    \label{fig:spatial domain rgb pearson vs l2 physical}
	\end{subfigure}		
	\\ % --- raw 3 ----
	\begin{subfigure}{0.49\columnwidth}
		\centering
		\captionsetup{justification=centering}		
        \includegraphics[width=0.975\linewidth,valign=t]{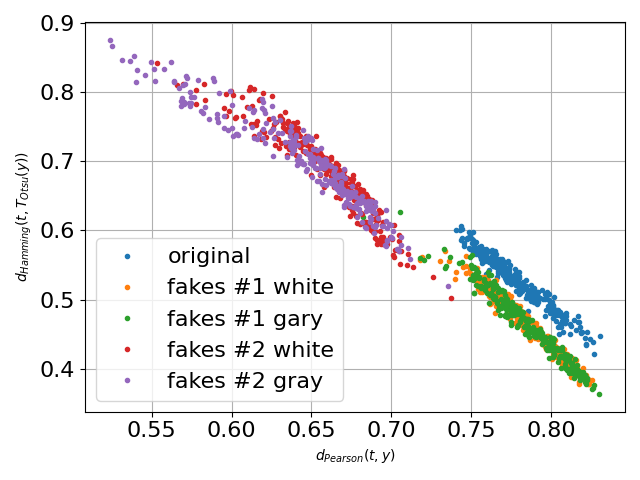}
	    \caption{Pearson correlation vs Hamming distance \\ with respect to the digital templates/references.}
	    \label{fig:spatial domain gray pearson vs xor otsu digital}
	\end{subfigure}		
	\begin{subfigure}{0.49\columnwidth}
		\centering
		\captionsetup{justification=centering}		
        \includegraphics[width=0.975\linewidth,valign=t]{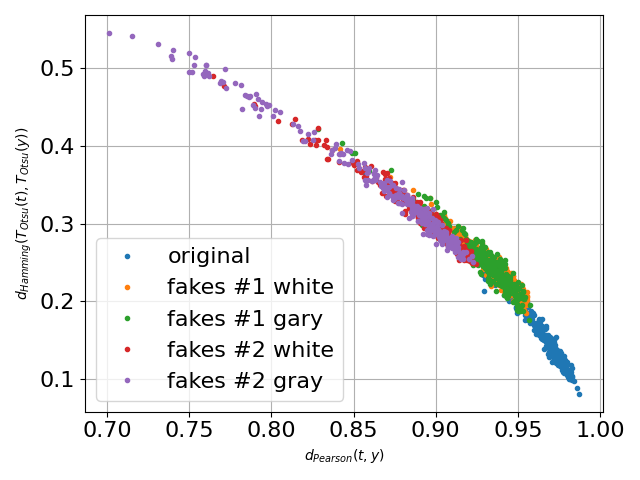}
	    \caption{Pearson correlation vs Hamming distance \\ with respect to the physical references.}
	    \label{fig:spatial domain rgb pearson vs xor otsu physical}
	\end{subfigure}		
	\\
    \caption{The 2D PGC separability in spatial domain with respect to the $\ell_2$, $\ell_1$, Hamming distances and Pearson correlation between the references (digital or physical) and the corresponding printed codes (original and fakes) (part 2).}
    \label{fig:spatial domain two metric part 2}        
\end{figure}

% ---------------------------------
